# Supplementary material for: Triple-entry Accounting, Blockchain and Next of Kin: Towards a Standardisation of Ledger Terminology
Source: arXiv:2101.02632 source file (2025-04-08)
Supplement: Supplementary file 1 [file appendix_firms.tex]

\begin{table}[t]
\centering
\label{table:wacc}
\caption{Variables used to compute firms' \ac{DCF}. We set $\it{MarketReturn}$ to the average yearly market return: 10\%. We use Damodaran's industry $\beta$ and $\it{TaxRate}$ \citep{damodaran_beta, damodaran_tax_rate}. The cost of debt $R_d$ was retrieved from the firms' 10-K document. The cost of capital $R_e$ is the product of $\beta$ and $\it{MarketReturn}$. Finally, we compute ${\it{WACC}}$ with \autoref{eq:wacc}.}
\scriptsize
\begin{tabular}{@{}rrrrrrcrrrrrr@{}}
\toprule
\phantom{abc} & \multicolumn{1}{c}{$\beta$} &
\phantom{abc} & \multicolumn{1}{c}{$Market Return$} &
\phantom{abc} & \multicolumn{1}{c}{$R_d$} &
\phantom{abc} & \multicolumn{1}{c}{$R_e$} &
\phantom{abc} & \multicolumn{1}{c}{$Tax Rate$} &
\phantom{abc} & \multicolumn{1}{c}{$WACC$} \\ \midrule

\textbf{BAC} & 1.12 && \textit{10\%} && \textit{2.85\%} && \textit{11.20\%} && \textit{14.69\%} && \textit{10.59\%} \\
\textbf{BLK} & 1.05 && \textit{10\%} && \textit{2.10\%} && \textit{10.50\%} && \textit{13.37\%} && \textit{10.46\%} \\
\textbf{BRK.B} & 1.05 && \textit{10\%} && \textit{3.30\%} && \textit{10.50\%} && \textit{13.37\%} && \textit{10.47\%} \\
\textbf{C} & 1.12 && \textit{10\%} && \textit{2.88\%} && \textit{11.20\%} && \textit{14.69\%} && \textit{10.08\%} \\
\textbf{CBOE} & 1.05 && \textit{10\%} && \textit{2.63\%} && \textit{10.50\%} && \textit{13.37\%} && \textit{10.47\%} \\
\textbf{ICE} & 1.12 && \textit{10\%} && \textit{3.00\%} && \textit{10.50\%} && \textit{13.37\%} && \textit{10.42\%} \\
\textbf{MS} & 1.12 && \textit{10\%} && \textit{2.90\%} && \textit{10.50\%} && \textit{13.37\%} && \textit{9.20\%} \\
\textbf{NDAQ} & 1.12 && \textit{10\%} && \textit{3.75\%} && \textit{10.50\%} && \textit{13.37\%} && \textit{10.28\%} \\
\textbf{WFC} & 1.05 && \textit{10\%} && \textit{2.37\%} && \textit{11.20\%} && \textit{14.69\%} && \textit{10.97\%} \\

\bottomrule
\end{tabular}
\end{table}
